# Supplementary material for: Frame Representation Hypothesis: Multi-Token LLM Interpretability and Concept-Guided Text Generation
Source: arXiv:2412.07334 source file (2024-12-12)
Supplement: Supplementary file 1 [file liegroupgeo.tex]

\section{Lie Group Geometry}

A $\numbers$-frame is a set of $\numbers$ linearly independent $\dimension$-dimensional vectors from euclidean space $\vectorspace$, which is represented by a matrix from $\matrixspace$. The Stiefel manifold $\stiefelmanifold{}$ is the set of all orthonormal $\numbers$-frames in $\dimension$-dimensional euclidean vector space $\vectorspace$~\cite[p.~4]{edelman1998geometry}

    \begin{equation}
        \stiefelmanifold{} \coloneqq \set{\mat{F} \in \matrixspace \mid \mat{F}^\top \mat{F} = \mat{I}_\numbers}
    \end{equation}

Furthermore, a $\numbers$-frame can represent more than a fixed set of vectors, but a subspace basis $\subspacemat{F} = \Span(\mat{F}) \subset \vectorspace$. Analogously, the Grassmann manifold $\Grassmann(\numbers, \dimension)$ is the set of all $\numbers$-dimensional subspaces of $\dimension$-dimensional euclidean vector space $\vectorspace$~\cite[p.~4]{Bendokat_2024}

    \begin{equation}
        \Grassmann(\numbers, \dimension) \coloneqq \set{\mat{F}\mat{F}^\top \in \squarematrixspace \mid \mat{F} \in \stiefelmanifold{}}
    \end{equation}

Particularly, these can be taken as manifolds because they can be represented as Lie groups. The subset of all invertible matrices from $\squarematrixspace$ makes the General Linear Group $\GL(\dimension) \coloneqq \set{\mat{A} \in \squarematrixspace \mid \det(\mat{A}) \neq 0}$, and its subset of orthogonal matrices is called the Orthogonal Group $\Or(\dimension) = \set{\mat{Q} \in \GL(\dimension) \mid \mat{Q}^\top \mat{Q} = \mat{I}_\dimension}$. An orthonormal $\numbers$-frame can be made by taking only the first $\numbers$ columns of an orthogonal matrix, so the space of all orthonormal frames becomes the quotient space $\stiefelmanifold{} \simeq \orthogonalframegroup$. Analogously, the space of all $\numbers$-dimensional subspaces becomes the quotient space $\Grassmann(\numbers, \dimension) \simeq \subspacegroup$. Whereas these are considered two distinct objects, frames and subspaces can be unified by introducing the concept of flags.~\cite{edelman1998geometry,Bendokat_2024}

\begin{definition}[Flag]
    A flag $\flag{F} = \{ \subspace{F}_i \}_{i = 1}^{\flagtypesize}$ is a nested sequence of subspaces 
    
    \begin{equation}
        \varnothing \subset \subspace{F}_1 \subset \subspace{F}_2 \subset \dots \subset \subspace{F}_\flagtypesize \subset \vectorspace
    \end{equation}
\end{definition}

In matrix space, $\flagmat{F}_{(\flagtype)}$ represents a flag of type $\flagtype$, $0 < \numbers_1 < \numbers_2 < \dots < \numbers_\flagtypesize < \dimension$, built from sub-frames within an orthonormal $\numbers_\flagtypesize$-frame $\mat{F}$
\begin{equation}
    [\mat{F}_{\dots \numbers_1}] \subset [\mat{F}_{\dots \numbers_2}] \subset \dots \subset [\mat{F}_{\dots \numbers_\flagtypesize}] = \subspacemat{F} \subset \vectorspace
\end{equation}
where $\mat{F}_{\dots \numbers_i}$ is the sub-frame containing the first $\numbers_i$ vectors of $\mat{F}$. We denote complete flags over $\mat{F}$ simply as $\flagmat{F}$, \ie, $\flagmat{F}_{(\completeflagtype)} = \flagmat{F}$

The set of all flags of type $(\flagtype)$ constitutes the Flag manifold $\genericflagmanifold$, but given flags are sequences of $\flagtypesize$ nested subspaces represented by a single matrix, the flag manifold must be a quotient space with $\flagtypesize + 1$ equivalences classes $$\genericflagmanifold \simeq \flaggroup$$ where $\numbers_0 = 0$ and $\numbers_{\flagtypesize + 1} = \dimension$~\cite{ye2022optimization}

Such a remark implies Flag manifolds generalize both Stiefel and Grassmann manifolds. Indeed, $\completeflagmanifold{} \simeq \orthogonalframegroup \simeq \stiefelmanifold{}$, while $\Flag(\numbers, \dimension) \simeq \subspacegroup \simeq \Grassmann(\numbers, \dimension)$. Therefore, while the subspace representation is invariant to swaps of vectors (rotations), the flag introduces regions of invariance because it is a nested sequence, so some vectors can swap with others but they are not free to swap with any other vector. In turn, this also adds a notion of ordering to the vectors and subspaces, making it equivalent to a frame in the complete case. Notice however, this is an equivalence in how these entities are represented in the orthogonal group, while the underlying geometric object can still be regarded as distinct, \eg, a frame is not necessarily a sequence of orthonormal 1-dimensional subspace, but both are represented by the same matrix.
